# Supplementary material for: Conditional Training with Bounding Map for Universal Lesion Detection
Source: arXiv:2103.12277 source file (2021-03-23)
Supplement: Supplementary file 1 [file Supplementary487.pdf]

# Supplementary Materials for Conditional Training with Bounding Map for Universal Lesion Detection

Paper ID 487

Anonymous Organization

## 1 Visualization of detection results

We randomly choose four CT images from DeepLesion dataset [1] to visually compare the detection results of AlignShift [2] w/ and w/o our methods. As shown in Fig. 1, the number of high-classification-score FP predictions is decreased (a&c&d) and more accurate results (b) are obtained with the help of our method.

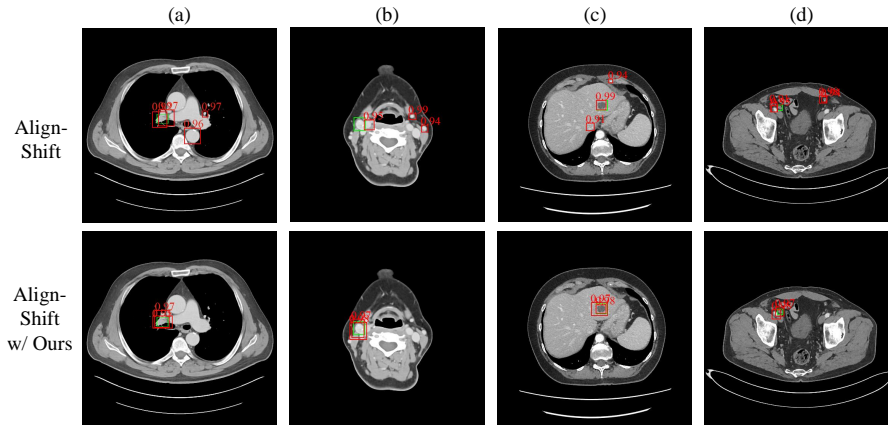

**Fig. 1.** High score BBoxes prediction (above 0.9) of AlignShift [2] with or without proposed method on test images. Red and green BBoxes denotes predicted BBoxes and GT BBoxes, respectively. The scores are marked above the BBoxes.

## 2 The number of positive anchors based on IoU

We compute the number of matched positive anchors per image (a in Fig. 2) and per GT BBoxes (b in Fig. 2) based on the IoU mechanism. The IoU threshold is set as 0.7. As shown in Fig. 2, the number of positive anchors is very few

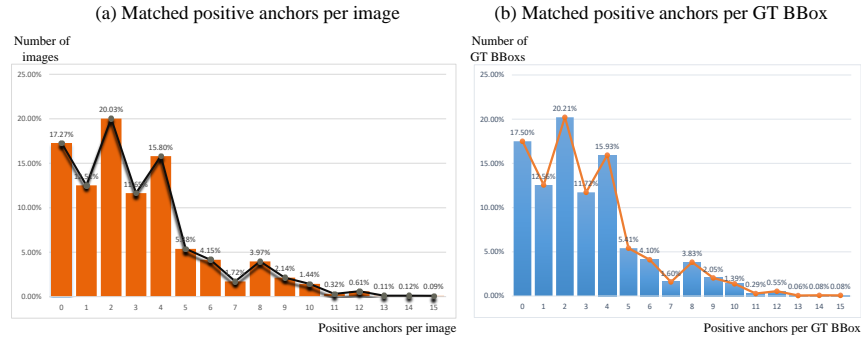

**Fig. 2.** We count the number of matched positive anchors per image (a) and per GT BBoxes (b) based on the IoU mechanism.

for both per-image manner and per-GT-BBox manner. More than 70% of GT-BBoxes (or images) match no greater than four positive anchors. This will cause a high imbalance of positive anchors v.s. negative anchors during training.

## References

1. K. Yan, X. Wang, L. Lu, L. Zhang, A. P Harrison, M. Bagheri, and R. M Summers. Deep lesion graphs in the wild: relationship learning and organization of significant radiology image findings in a diverse large-scale lesion database. In *IEEE CVPR*, pages 9261–9270, 2018.
2. Jiancheng Yang, Yi He, Xiaoyang Huang, Jingwei Xu, Xiaodan Ye, Guangyu Tao, and Bingbing Ni. Alignshift: bridging the gap of imaging thickness in 3d anisotropic volumes. In *MICCAI*, pages 562–572. Springer, 2020.
